# Supplementary material for: Deep vacancy induced low-density fluxional interfacial water
Source: arXiv:2107.02483 source file (2021-07-06)
Supplement: Supplementary file 1 [file supplementary_materials.pdf]

# Supporting Information: Deep vacancy induced low-density fluxional interfacial water

Keyang Liu,† Jianqing Guo,‡ Weizhong Fu,† and Ji Chen*,†

†*School of Physics, Peking University, Beijing 100871, People's Republic of China*

‡*International Center for Quantum Materials, School of Physics, Peking University, Beijing 100871, People's Republic of China*

¶ *Collaborative Innovation Center of Quantum Matter, Beijing 100871, People's Republic of China*

E-mail: ji.chen@pku.edu.cn

# OUTLINE

The supporting information contains additional data and convergence tests to support the conclusions of the main text, including convergence tests (Fig. S1, Fig. S2), computational details of order parameter (Fig. S4), tests of results on methods (Fig. S3, Fig. S9, Fig. S10), tests of one-interface model (Fig. S15), extended analyses (Fig. S5, Fig. S6, Fig. S11, Fig. S12), and additional data (Fig. S7, Fig. S8, Fig. S13, Fig. S14).

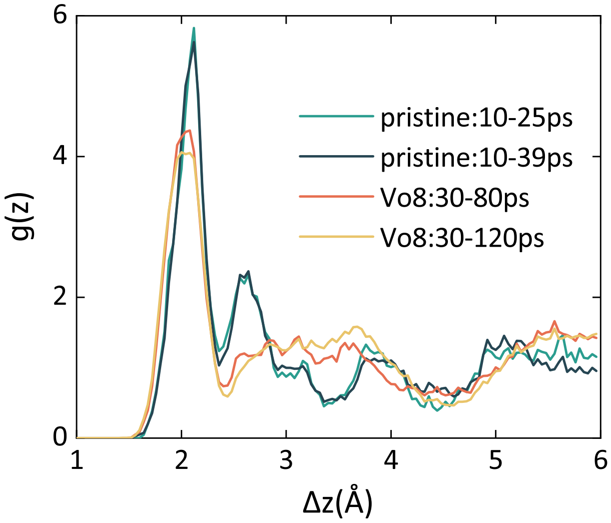


Figure S1: **Convergence tests for the pristine and the $V_O8$ systems.** All trajectories discussed in the main text have reached equilibrium and here in Fig. S1 are two examples representing one high-density structure (pristine) and one low-density structure ($V_O8$). Each trajectory, after reaching equilibrium, is collected into a short and a long time scale. The consistency of g(z) profiles in two time windows confirms the convergence.

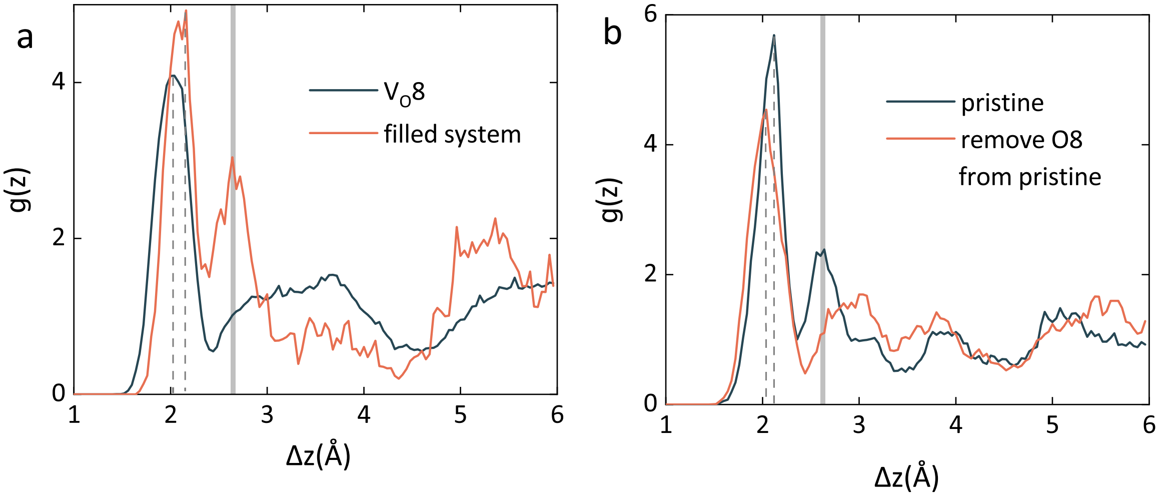


Figure S2: **Check tests for different combinations of interfacial water structure and substrate.** Two tests are carried out, initializing by filling the vacancy of equilibrated $V_O8$ system (a) and removing an 8th layered oxygen from equilibrated pristine system (b). Density reduction is confirmed.

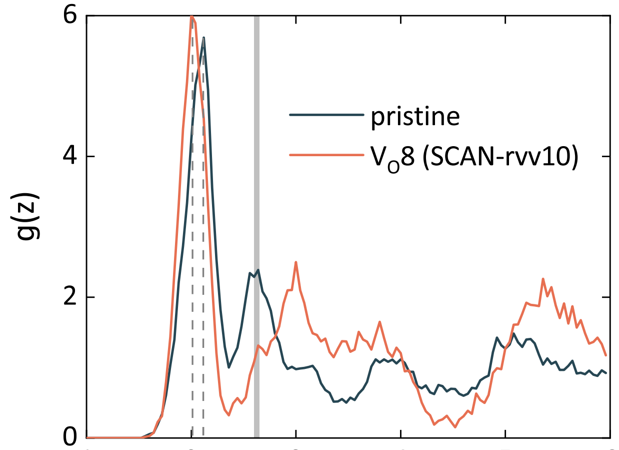


Figure S3: **Tests of g(z) in $V_O8$ system with SCAN-rvv10 exchange correlation functional.** Density reduction is confirmed.

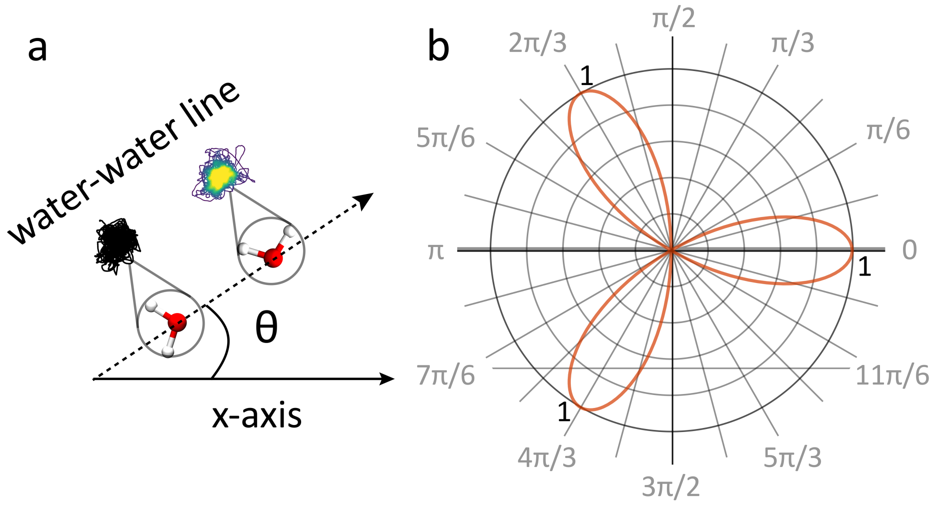


Figure S4: **Details of the order parameter $\sigma$.** (a) Water-water line is a vector from a molecule on $Ti_{5c}$ to a molecule on $O_{2c}$. $\theta$ is defined as the angle between the molecule-molecule line and the x-axis. (b) $\sigma = \cos(3\theta)$ in polar coordinate. When $\theta = 0$, $\theta = \frac{2}{3}\pi$ and $\theta = \frac{4}{3}\pi$, $\sigma$ gets a maximum value of 1. In contrast, $\sigma$ has a minimum value of -1 in directions at $\theta = \frac{1}{3}\pi$, $\theta = \pi$, and $\theta = \frac{5}{3}\pi$. The maximum angle $\theta$ is 120 degrees, which is obtained from the distribution of orderly adsorbed water molecules.

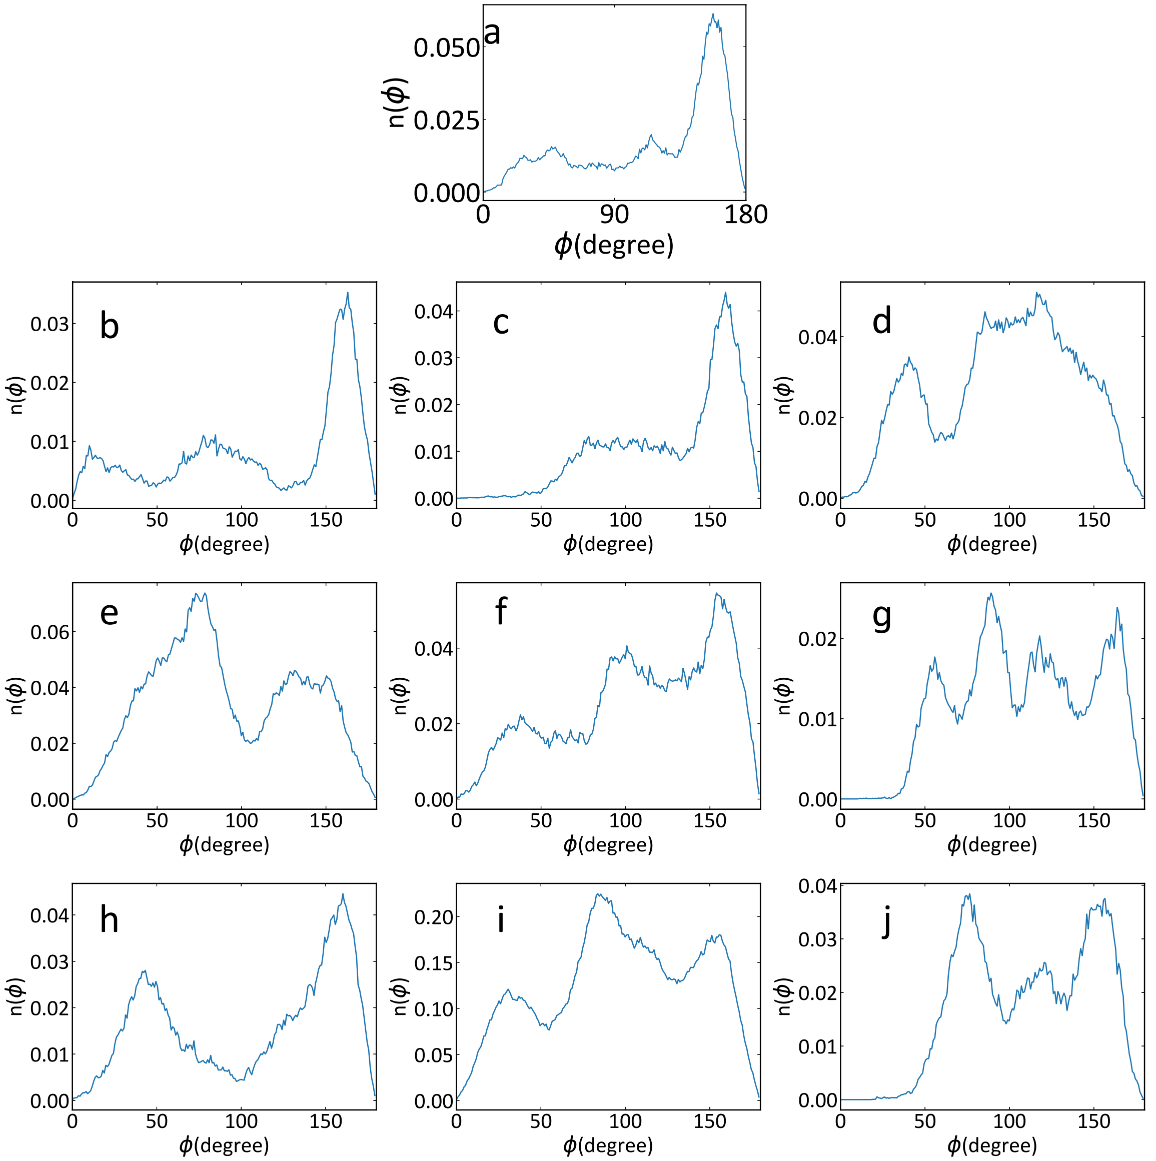


Figure S5: **Water orientation distribution.** The distribution of water orientation $\phi$ for all ten systems. (a) represents the pristine system and (b-j) indicate defected systems from $V_O1$ to $V_O9$, respectively. $\phi$ is the angle between surface normal and the orientation of a water molecule, which is defined as the vector from $O_W$ to the center of two hydrogen atoms. Water molecules considered are the same as those shown in the projected trajectories in the main text. For the high-density model, the characteristic peak is at about 160 degrees as a result of the double-leg hydrogen bonding to $O_{2c}$s. In the low-density structures, the orientation of water molecules features multiple peaks.

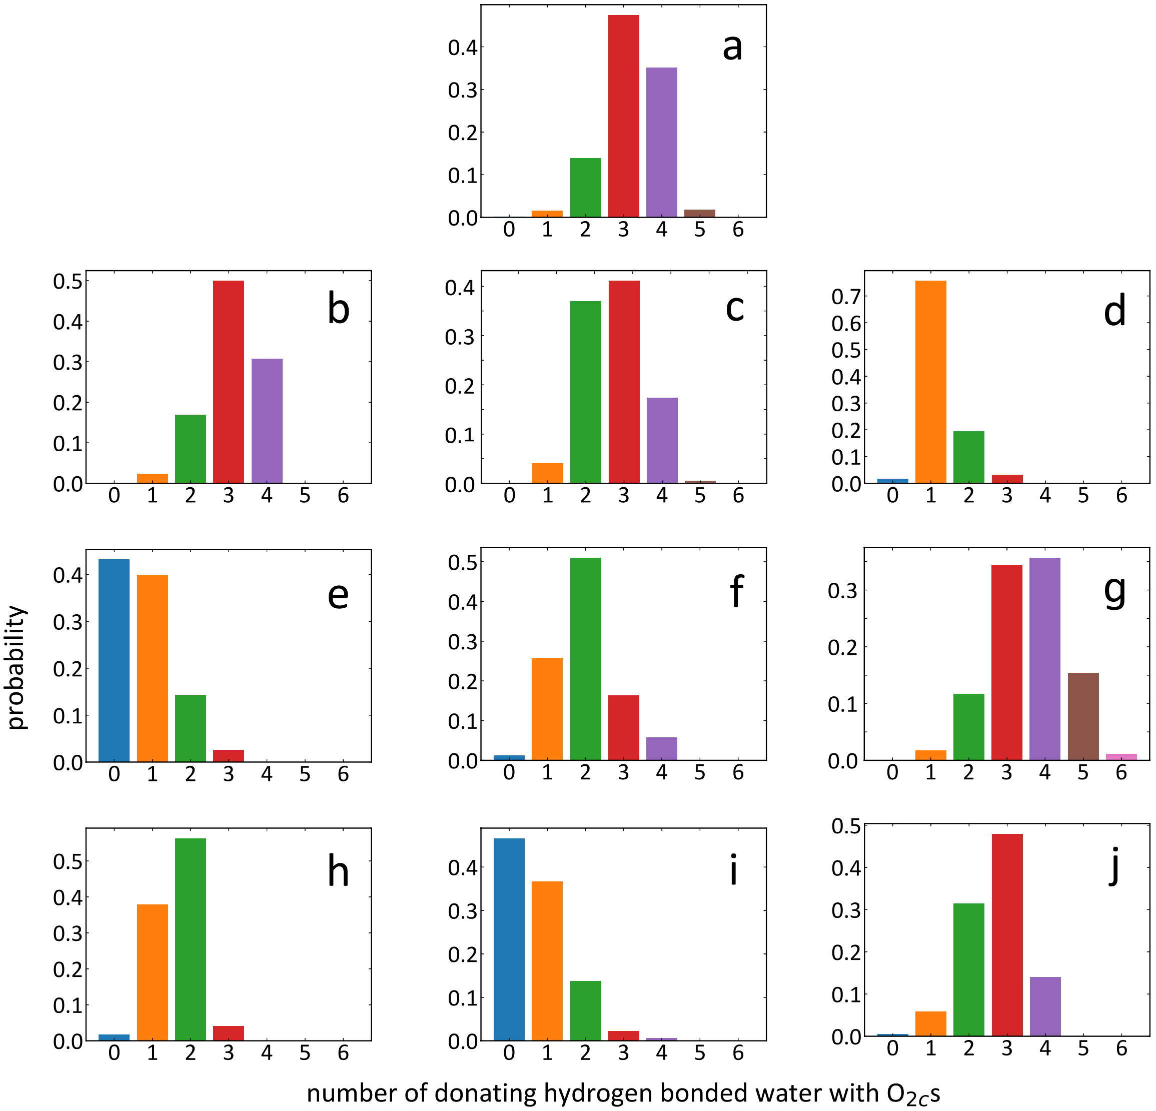


Figure S6: **Distribution of the number of donating hydrogen bonded water with $O_{2c}$s.** (a) represents the pristine system and (b-j) indicate defected systems with $V_O1$ to $V_O9$, respectively. The number of donating hydrogen bonded water are counted within a distance of 2 Å to $O_{2c}$s. high-density interfacial water features more hydrogen atoms near one $O_{2C}$ site to form hydrogen bonds. The low-density models generally feature less hydrogen bonds around one $O_{2c}$ site.

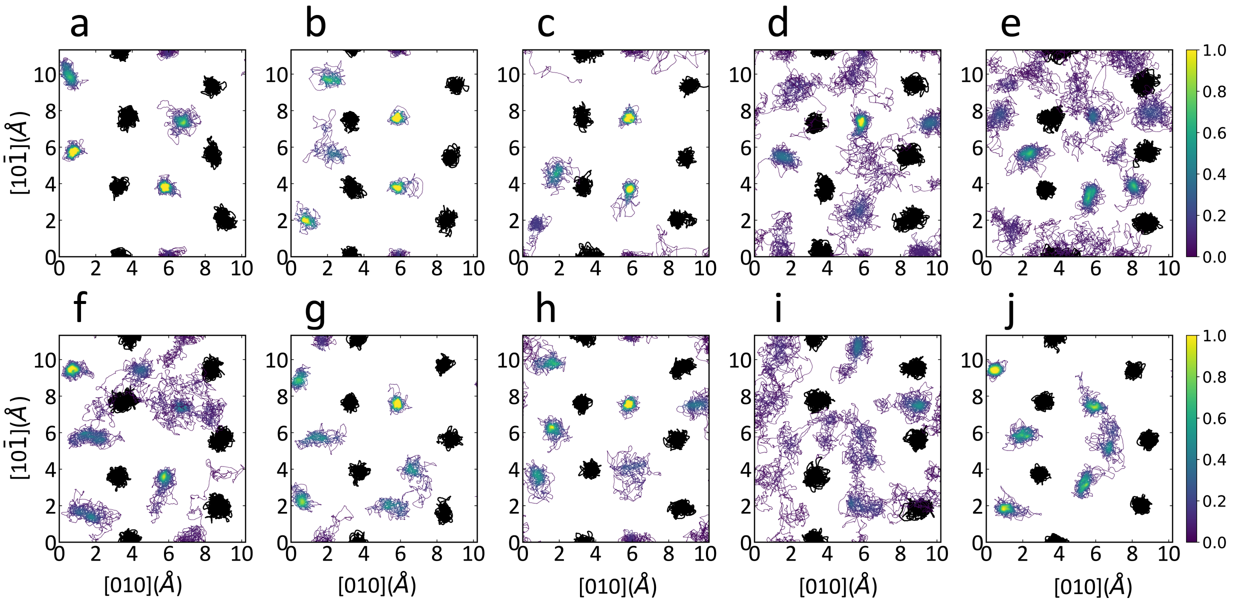


Figure S7: **Projected trajectories of interfacial water molecules in x-y plane.** (a) The pristine system and (b-j) defected systems with $V_O1$ to $V_O9$ respectively. The position of water is identified by the oxygen atom. An uniform sequential colormap of viridis represents the lateral distribution density of a water molecule adsorbed on $O_{2c}$. Water molecules on $Ti_{5c}$ are plotted with black lines. Water molecules within the first shell, with a cutoff radius of 3 Å from $O_{2c}$ and 2.5 Å from $Ti_{5c}$, are taken into account.

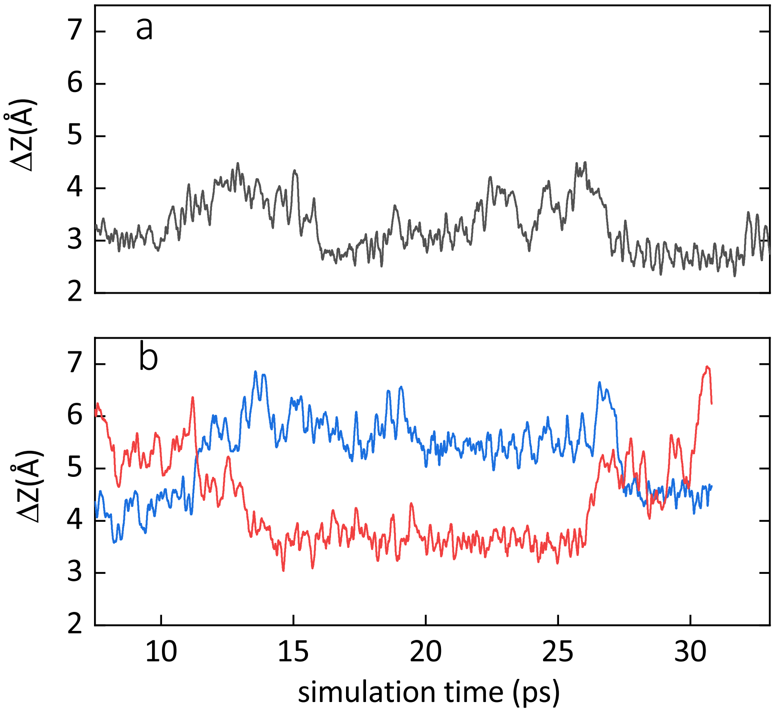


Figure S8: **Fluxional properties of interfacial water.** The plots show relative vertical position (in Å ) of water molecules as function of time. These trajectories are from systems with $V_O4$ (a) and $V_O5$ (b) and the reference point z=0 is chosen as the average z position of $Ti_{5c}$. The trajectories srhow large variations of contact layer water and exchanges between contact water and bulk liquid.

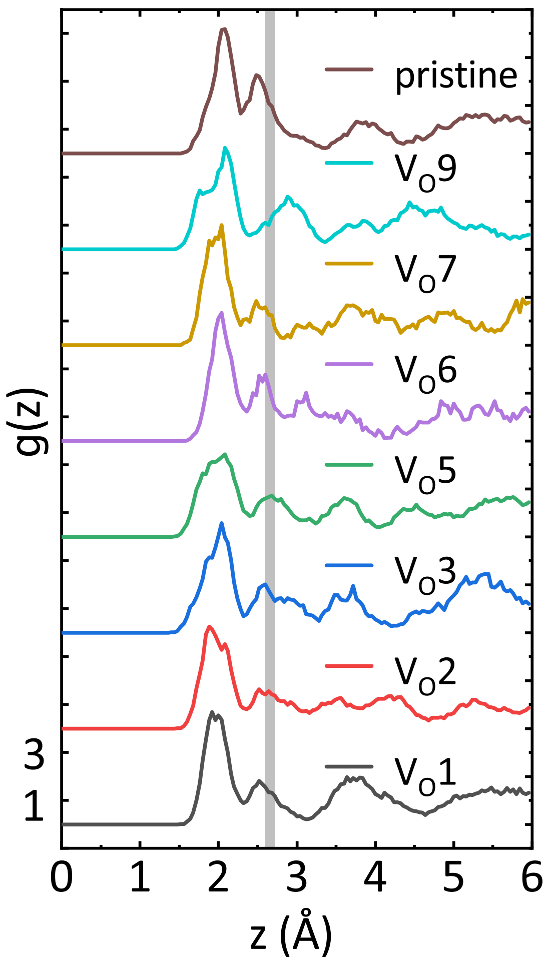


Figure S9: **g(z) profiles of 8 systems with Hubbard U corrections.** U=3.9 eV is used. The g(z) profiles show the sensitivity of interfacial structure to the the position of vacancy.

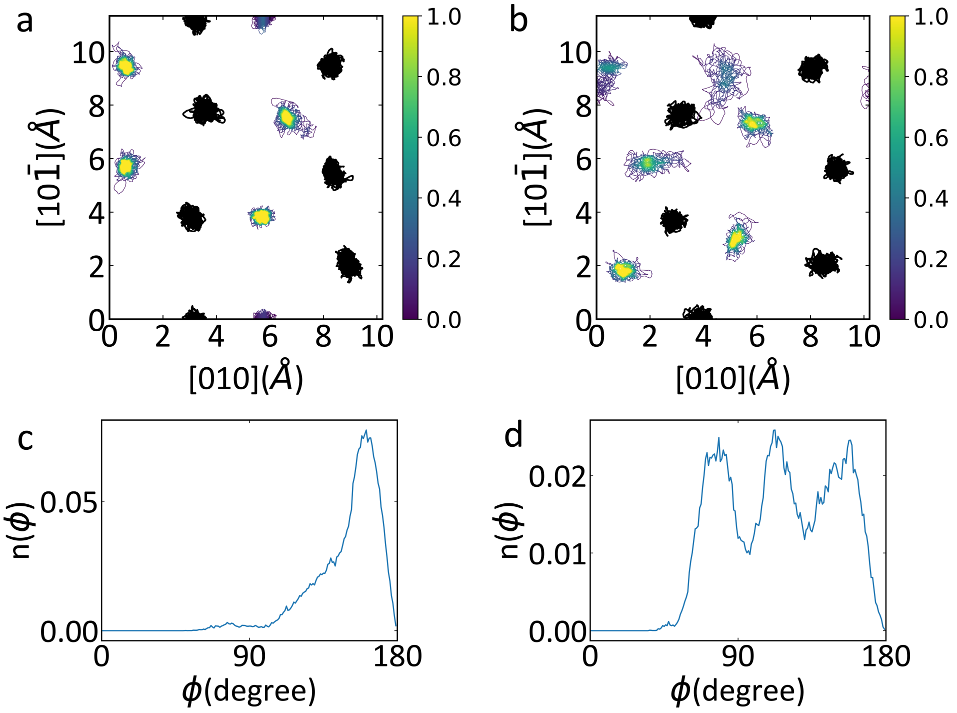


Figure S10: **Calculations with Hubbard U correlations.** U=3.9 eV is used. (a-b) The projected trajectories in the pristine system and $V_O9$ system, respectively. (c-d) The orientation distribution of water molecules on $O_{2c}$s in the pristine system and the $V_O9$ system, respectively. These analyses support the results that a deep vacancy in substrate can induce significant density reduction and increased flexibility of interfacial water.

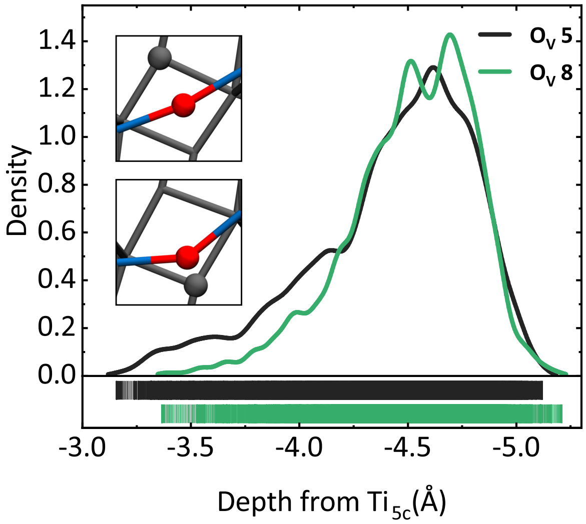


Figure S11: **Position distribution density of a dangling oxygen atom (with rug plot) in systems with $V_O5$ and $V_O8$.** The green line indicates the trajectory with $V_O8$, while the black line represents the trajectory with $V_O5$. Side-view snapshots of the structure around initial $V_O$ site (grey balls) are shown in the insets, where the upper and the lower insets come from systems with $V_O5$ and $V_O8$, respectively.

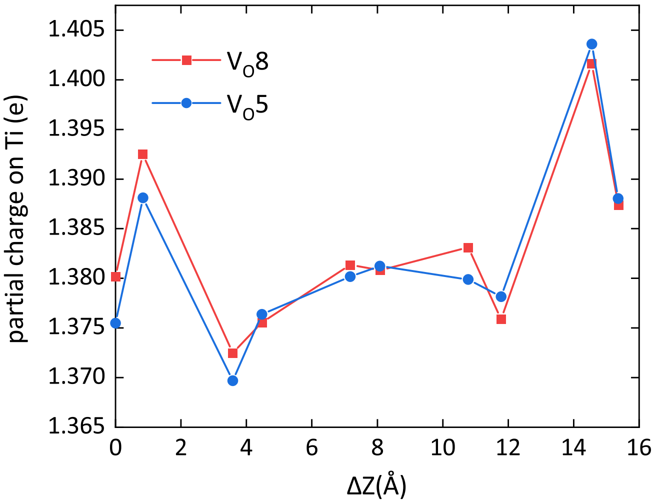


Figure S12: **Charge distribution (a.u.) in the substrates of $V_O5$ (a) and $V_O8$ (b).** The charge distribution is an average value of the partial charge of six Ti atoms in each layer calculated by the Bader method.

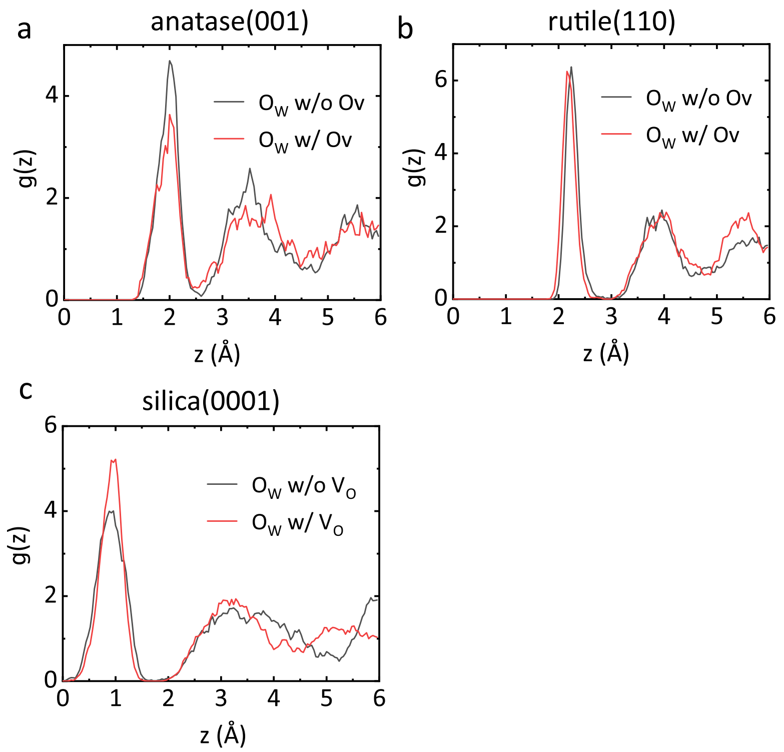


Figure S13: **Results on other systems.** (a-c) g(z) profiles of water oxygen ($O_W$) for systems of anatase (001), rutile (110) and silica (0001), respectively. Comparisons are made between systems with and without a deep oxygen vacancy ($V_O$). In all these three systems, g(z) profiles show minor differences in water distribution with and without the deep oxygen vacancy. On rutile (110) the interfacial water does not dissociate. On anatase (001), water dissociates and leads to hydroxylation of the surface. On silica (0001), the surface model is built with a hydroxylated model.

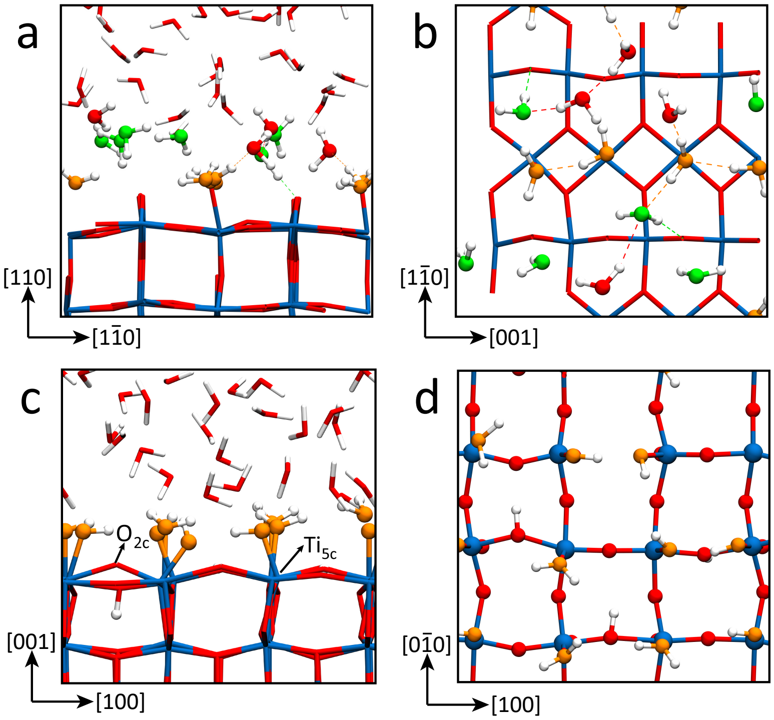


Figure S14: **Side view and top view of other $TiO_2$ facets.** (a) A side view and (b) a top view of rutile (101) interfacial water. The oxygen and titanium atoms are represented by red and blue, respectively. Orange and green spheres highlight water molecules in the contact layer, respectively on $Ti_{5c}$ and $O_{2c}$ sites. (c) A side view and (d) a top view of the anatase (001) interfacial water. Orange spheres highlight water molecules or species in the contact layer.

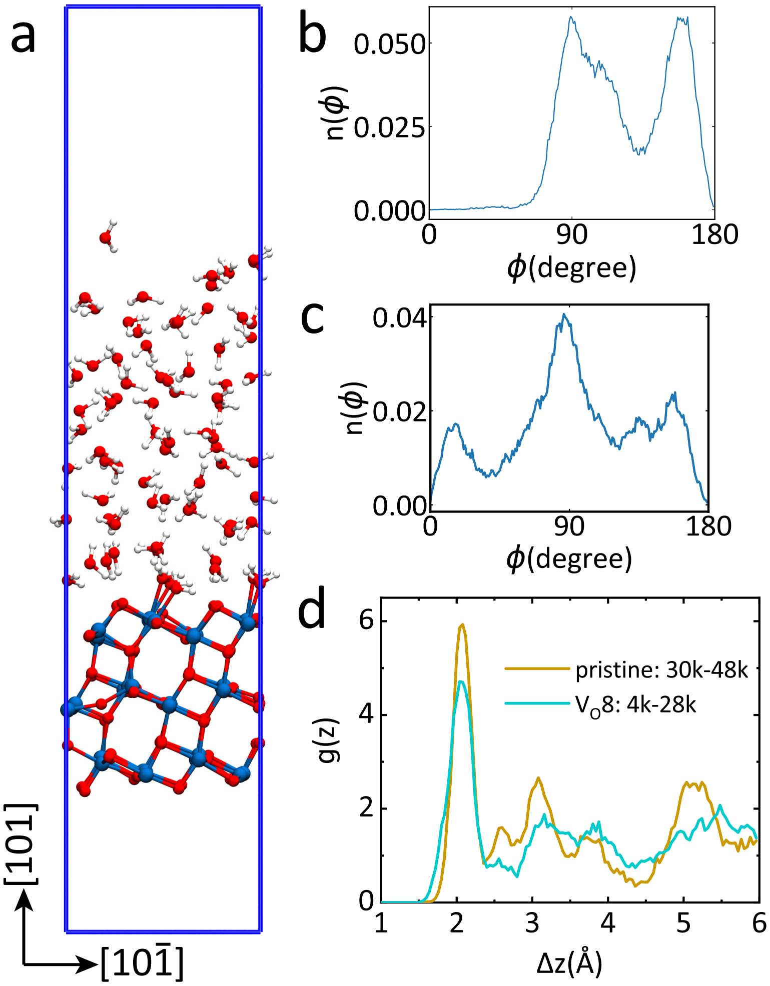


Figure S15: **Simulations with the one-interface model.** (a) A side view of the snapshot to show the simulation supercell, which contains a 15 Å vacuum slab. (b-c) orientation distribution of interfacial water on bridging oxygen. (d) g(z) profiles of the pristine and the $V_O8$ substrates. The reference point (z=0) is chosen as the average z value of all $Ti_{5c}$s of the whole trajectory. Density reduction is observed in $V_O8$ system compared with the pristine system.
